# Supplementary material for: Core Higher-Order Session Processes: Tractable Equivalences and Relative Expressiveness
Source: arXiv:1502.02585 source file (2015-02-10)
Supplement: Supplementary file 1 [file app-negative.tex]

\section{Negative Result}
\label{app:neg}

\begin{theorem}\rm
	There is no encoding $\enco{\map{\cdot}, \mapt{\cdot}, \mapa{\cdot}}: \HOp \longrightarrow \HOp^{\minussh}$
	that enjoys operational correspondence and full abstraction.
\end{theorem}

\begin{proof}
	Let $\horel{\Gamma_1}{\Delta_1}{P_1}{\not\wb}{\Delta_2}{P_2}$
	with $P = \breq{a}{s} \inact \Par \bacc{a}{x} P_1 \Par \bacc{a}{x} P_2$ and
	let $\Gamma; \emptyset; \Delta \proves P \hastype \Proc$.
	Assume also a encoding
	$\enco{\map{\cdot}, \mapt{\cdot}, \mapa{\cdot}}: \HOp \longrightarrow \HOp^{\minussh}$
	that enjoys
	operational correspondence and full abstraction.

	From operational correspondence we get that:
	\begin{eqnarray*}
		P \red P_1 \Par \bacc{a}{x} P_2 &\textrm{implies}& \map{P} \red \map{P_1 \Par \bacc{a}{x} P_2}\\
		P \red P_2 \Par \bacc{a}{x} P_1 &\textrm{implies}& \map{P} \red \map{P_2 \Par \bacc{a}{x} P_1}
	\end{eqnarray*}

	From the fact that
	$\horel{\Gamma_1}{\Delta_1}{P_1}{\not\wb}{\Delta_2}{P_2}$
	we can derive that
	\[
		\horel{\Gamma_1'}{\Delta_1'}{P_1 \Par \bacc{a}{x} P_2}{\not\wb}{\Delta_2'}{P_2 \Par \bacc{a}{x} P_1}
	\]
	From Corollary~\ref{cor:tau_inert} we know that
	\begin{eqnarray*}
		\horel{\mapt{\Gamma}}{\mapt{\Delta}}{\map{P}}{\wb}{\mapt{\Delta_1'}}{\map{P_1 \Par \bacc{a}{x} P_2}}\\
		\horel{\mapt{\Gamma}}{\mapt{\Delta}}{\map{P}}{\wb}{\mapt{\Delta_2'}}{\map{P_2 \Par \bacc{a}{x} P_1}}
	\end{eqnarray*}
	\noi thus
	\[
		\horel{\mapt{\Gamma}}{\mapt{\Delta_1'}}{\map{P_1 \Par \bacc{a}{x} P_2}}{\wb}{\mapt{\Delta_2'}}{\map{P_2 \Par \bacc{a}{x} P_1}}
	\]
	From here we conclude that the full abstraction property does not hold,
	which is a contradiction.
	\qed
%	so there is no mapping $\map{\cdot}: \pHO \longrightarrow \spi$ that enjoys
%	the operational correspondence and full abstraction properties.
\end{proof}
